# Supplementary material for: Boosting Camera Motion Control for Video Diffusion Transformers
Source: arXiv:2410.10802 source file (2024-10-14)
Supplement: Supplementary file 1 [file appendix.tex]

\clearpage
\appendix
\section{Appendix}
You may include other additional sections here.
